# Supplementary material for: Magnetization dynamics affected by phonon pumping
Source: arXiv:2202.03331 source file (2022-02-07)
Supplement: Supplementary file 1 [file 220204_ME_coupling_SM.pdf]

# Supplemental Material: Magnetization dynamics affected by phonon pumping

Richard Schlitz,[1,2,*] Luise Siegl,[3,2] Takuma Sato,[4] Weichao Yu,[5,6,4] Gerrit E. W. Bauer,[4,7,8] Hans Huebl,[9,10,11] and Sebastian T. B. Goennenwein[3,2]

[1]*Department of Materials, ETH Zürich, 8093 Zürich, Switzerland*
[2]*Institut für Festkörper- und Materialphysik, Technische Universität Dresden and Würzburg-Dresden Cluster of Excellence ct.qmat, 01062 Dresden, Germany*
[3]*Department of Physics, University of Konstanz, 78457 Konstanz, Germany*
[4]*Institute for Materials Research, Tohoku University, Sendai 980-8577, Japan*
[5]*State Key Laboratory of Surface Physics and Institute for Nanoelectronic Devices and Quantum Computing, Fudan University, Shanghai 200433, China*
[6]*Zhangjiang Fudan International Innovation Center, Fudan University, Shanghai 201210, China*
[7]*AIMR and CSRN, Tohoku University, Sendai 980-8577, Japan*
[8]*Zernike Institute for Advanced Materials, Groningen University, Groningen, The Netherlands*
[9]*Walther-Meißner-Institut, Bayerische Akademie der Wissenschaften, 85748 Garching, Germany*
[10]*Physik-Department, Technische Universität München, 85748 Garching, Germany*
[11]*Munich Center for Quantum Science and Technology (MCQST), 80799 München, Germany*
(Dated: February 4, 2022)

## S1. ALTERNATIVE EVALUATION PROCEDURE

An alternative approach to evaluating the broadband FMR data based on a direct fit to the complex scattering parameter is presented in the following. To directly connect to the coupled resonator model and obtain the coupling strength, the impact of the microwave background signal must be removed before the data can be fit. This is accomplished by numerically differentiating the data as well as the coupled resonator model with respect to the frequency. This method is called derivative divide and was already used in previous broadband FMR experiment to remove the frequency and magnetic field dependent microwave background (however along the field axis) [1]. A side effect of this preprocessing of the data is that the phonon resonances are enhanced: Contributions to $S_{21}$ that vary rapidly in frequency (i.e. , the phonon resonances) become more pronounced, while slowly varying contributions (i.e. , the microwave background) are suppressed. To initialize the fit, we use the same approach as presented in the main text, i.e. we locate the FMR using a Gaussian fit to $|S_{21}|$ (see gray line in Fig. S1(a)). In the following, the first two phonon resonances that have a spacing from the Kittel mode $\geq 22\,\mathrm{MHz}$ are fitted with Lorentzians to determine the initial parameters for $\Delta\omega_\mathrm{p}$ (the spacing between the two phonon resonances), $\omega_{\mathrm{p},0}$ (the resonance frequency of the phonon resonance clostest to the FMR line) and the line width $\gamma_\mathrm{p}$ of the phonon resonance. We then fit the complex preprocessed data using the differentiated model. The processed data and the fit can be seen in Fig. S1(b). We would like to stress, that while this approach works and produces equivalent results if care is taken, some of the parameters show strong correlations. Consequently, it was not possible to automatically fit all of the experimental data reliably, in particular where the magnetoelastic coupling is weak. We attribute this issue to inhomogeneities in the YIG film along the CPW that lead to the broadening of the FMR and the presence of the first PSSW in the flank of the FMR line, which might lead to additional contributions to the phonon pumping. Nevertheless, in another work, a similar approach produced a very good fit of the complex response around the full FMR line at least for thick YIG films [2].

* richard.schlitz@mat.ethz.ch

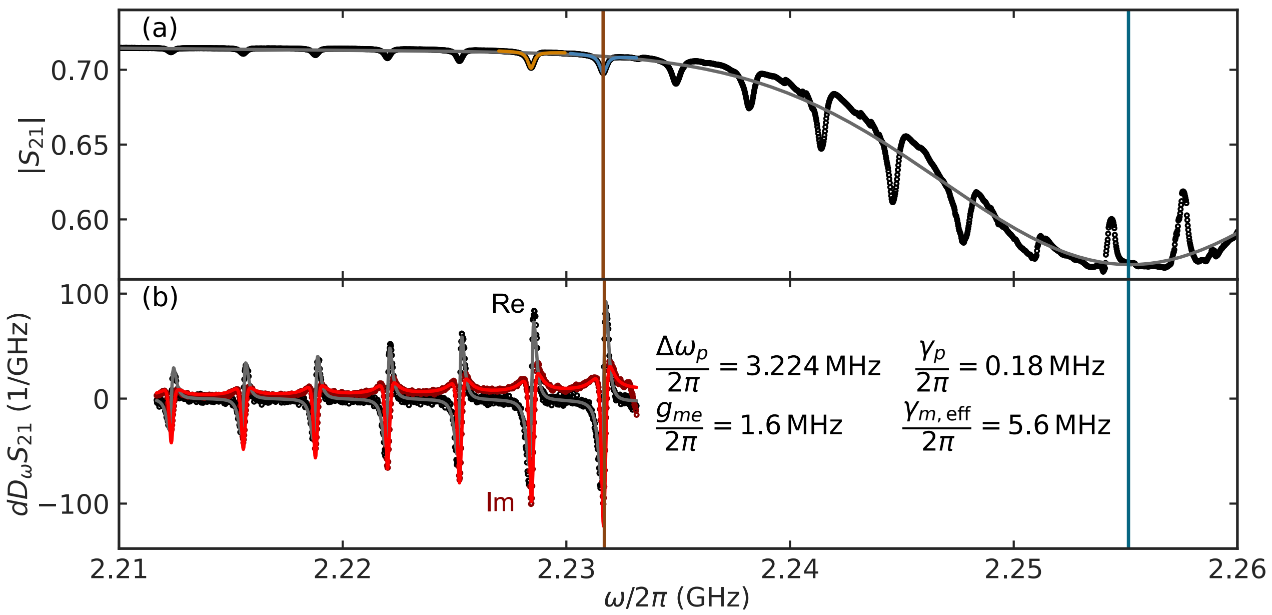


FIG. S1. (a) The $|S_{21}|(\omega)$ spectra are used to initialize the fit parameters for fitting the full complex response. In particular, the line width of the FMR line $\gamma_\mathrm{m}$ and the phonon resonance $\gamma_\mathrm{p}$ as well as the respective resonance positions $\omega_\mathrm{m}$ and $\omega_\mathrm{p}$ are extracted. (b) $S_{21}$ expected from the model (cf. Eq. (5) in the main text) is differentiated along the frequency axis and the resulting complex $\partial A_\mathrm{m}(\omega)/\partial\omega$ is fitted to a set of seven lines (simultaneously). The black line is the real part, while the red line shows the imaginary part of $S_{21}$. We find good quantitative agreement with the parameters that are extracted using the approach presented in the main text.

## S2. FULL SET OF FIT PARAMETERS AND DISCUSSION

In this section we list all of the different parameters that we obtain from our automatic fitting procedure (summarized in Fig. S2 and discuss their physical implications. In particular, the magnitude of the microwave background decays exponentially [panel (a)]. We point out that the dip seen around 4 GHz corresponds to a standing wave forming across the CPW structure, which has a length of $\sim 4\,\mathrm{cm}$. The height of the magnon resonance [panel (b)] shows a linear increase for increasing frequency. The latter is rooted in the measurement of our signal: $S_{21}$ has a component proportional to the voltage induced into the coplanar waveguide by the precessing magnetization $M(t)$. The inductance between the sample and the CPW is a constant given by the geometry, so that the voltage increases linearly with frequency due to the increase of $\partial M(t)/\partial t$ [3]. As a consequence, also the coupling strength between the CPW and the YIG sample (panel (d)) increases linearly with frequency.

The height of the phonon resonance shown in panel (e) exhibits a clear maximum around 3 GHz, vanishes around 6 GHz and then has another maximum around 9 GHz. It thus reflects the oscillating nature of the magnetoelastic coupling discussed in the main text. Note that this signature is observed for all the six fitted phonon lines and thus is independent of the distance of the phonon resonance from the FMR line. It is obvious, that the amplitude of the phonon resonance depends strongly on the separation from the FMR line. In particular, it roughly scales as the inverse of the separation from the FMR line, so that $h_mrp$ is strongly suppressed when increasing the separation. This is taken into account by the model when calculating the coupling strength shown in panel (g). The height of the phonon resonance is the dominant parameter when determining the coupling strength from the resonator model and thus will introduce the largest error.

Finally, one other parameter that we can determine from our fitting is the free spectral range, which is directly proportional to the sound velocity [see Eq. (1) in the main text]. The free spectral range is shown in panel (h). For a phonon band with linear dispersion, one expects a constant sound velocity, which is confirmed by our observation of a frequency independent free spectral range for frequencies up to 11 GHz.

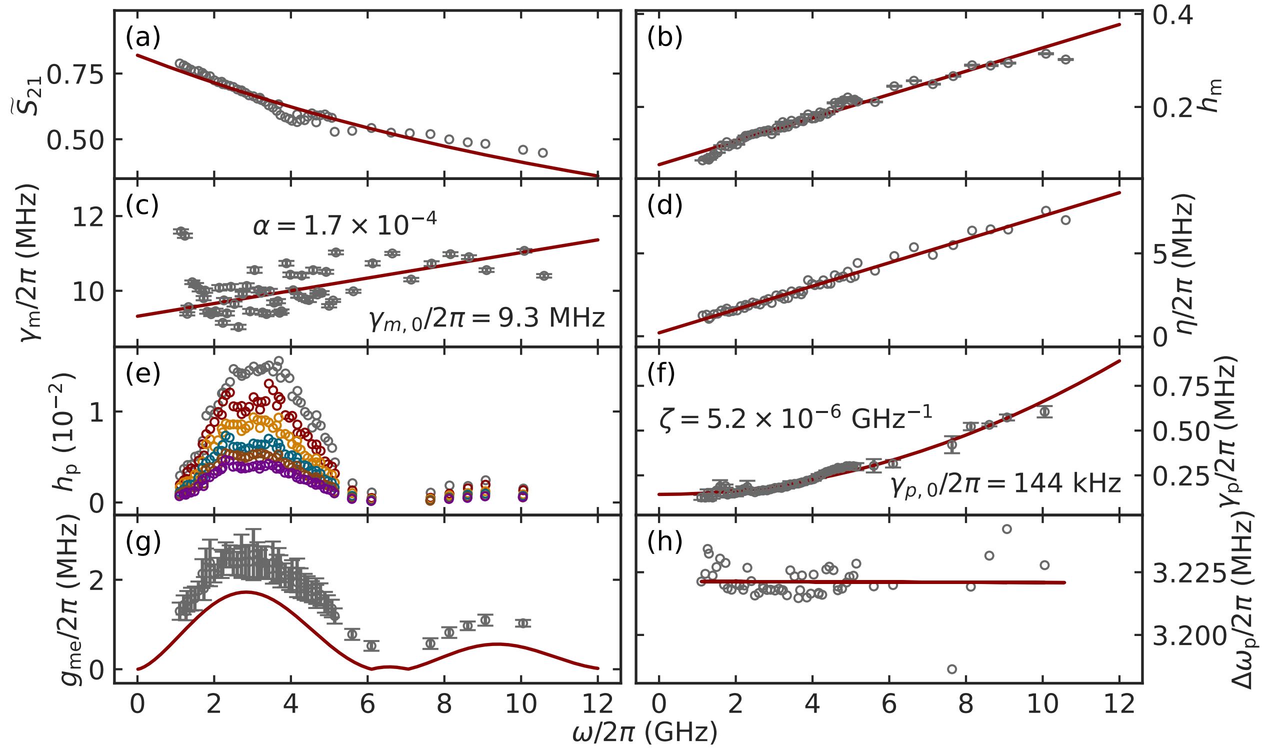


FIG. S2. (a) The microwave tranmission of the coplanar wavguide loaded with the sample in the absence of the FMR line decays roughly following an exponential. (b, c) Amplitude and half width at half maximum (HWHM) obtained from Gaussian fits to the FMR line. (d) The magnon-photon coupling strength between the CPW and the FMR in the YIG film decreases linearly by $\sim 20\,\%$ in the investigated frequency window. (e,f) Amplitude and width (HWHM) extracted from Lorentzian fits of the acoustic resonances. (g) The magnon-phonon coupling strength that parametrizes the spin pumping process and is discussed in more detail in the main text. (h) The free spectral range of the acoustic resonator does not depend on frequency, suggesting constant speed of sound in the investigated frequency range.

[1] H. Maier-Flaig, S. T. B. Goennenwein, R. Ohshima, M. Shiraishi, R. Gross, H. Huebl, and M. Weiler, Review of Scientific Instruments **89**, 076101 (2018).
[2] S. N. Polulyakh, V. N. Berzhanskii, E. Y. Semuk, V. I. Belotelov, P. M. Vetoshko, V. V. Popov, A. N. Shaposhnikov, A. G. Shumilov, and A. I. Chernov, Journal of Experimental and Theoretical Physics **132**, 257 (2021).
[3] M. A. W. Schoen, J. M. Shaw, H. T. Nembach, M. Weiler, and T. J. Silva, Physical Review B **92**, 184417 (2015).
